# Supplementary material for: COMPASS: A Unified Decision-Intelligence System for Navigating Performance Trade-off in HPC
Source: arXiv:2604.22688 source file (2026-04-27)
Supplement: Supplementary file 1 [file appendix.tex]

% \begin{table}[t]
\footnotesize
\centering
\setlength{\LTpre}{0pt}
\setlength{\LTpost}{0pt}
\begin{longtable}
{|P{0.10\textwidth}|P{0.14\textwidth}|P{0.40\textwidth}|P{0.32\textwidth}|}
\caption{Example queries and responses for each query type and dataset. \tzi{Ankur will remove it when all the results are done and shifted to the new table}}\label{tab:examples_sorted}\\
\hline
\textbf{Query Type} & \textbf{Dataset} & \textbf{Query} & \textbf{Response} \\
\hline
\endfirsthead

\hline
\multicolumn{4}{r}{\small\itshape Continued on next page}\\
\hline
\textbf{Query Type} & \textbf{Dataset} & \textbf{Query} & \textbf{Response} \\
\hline
\endhead

\hline
\multicolumn{4}{r}{\small\itshape Continued on next page}\\
\hline
\endfoot

\hline
\endlastfoot

% ------------------ RECO ------------------
\multirow{6}{*}{\texttt{\textbackslash reco}}
& Monet
& \cell{%
\textcolor{blue}{\textbf{Recommend a configuration where}}\\
\texttt{X = \{nettopo\_mesh\_coord\_Z: ?, nettopo\_mesh\_coord\_Y: ?, nettopo\_mesh\_coord\_X: ?\}}\\[0.25em]
\textcolor{blue}{\textbf{to achieve}}\\
\texttt{Y = \{X+\_SAMPLE\_GEMINI\_LINK\_INQ\_STALL: minimize, X+\_SAMPLE\_GEMINI\_LINK\_CREDIT\_STALL: minimize, X+\_SAMPLE\_GEMINI\_LINK\_USED\_BW: minimize\}}
}
& \cell{
\ankur{Only Link Stalls}
\texttt{X = \{nettopo\_mesh\_coord\_Z = 19.0, nettopo\_mesh\_coord\_Y = 11.0, nettopo\_mesh\_coord\_X = 22.0.\}} \\
Confidence: High (NLL: 0.00, OOD: 0.00, OOS: 0.00, MD: 0.00)
}\\ \cline{2-4}

& 
PM100
& \cell{%
\textcolor{blue}{\textbf{Recommend a configuration where}}\\
\texttt{X = \{cores\_per\_task: ?, num\_cores\_req: ?, num\_nodes\_req: ?, mem\_req: ?, time\_limit: ?\}}\\[0.25em]
\textcolor{blue}{\textbf{to achieve}}\\
\texttt{Y = \{node\_power\_consumption: minimize, mem\_power\_consumption: minimize, cpu\_power\_consumption: minimize, job\_state: completed, num\_gpus\_req = 4\}}
}
& \cell{%
\texttt{X = \{num\_cores\_req = 64, mem\_req = 128GB\}}\\
Confidence: Moderate (NLL: 0.28, OOD: 0.15, OOS: 0.22, MD: 0.19)
}\\ \cline{2-4}

& Butter-E
& \cell{%
\textcolor{blue}{\textbf{Recommend}} a configuration\\
\texttt{X = \{is\_gpu: True, dataset: 'mnist', depth: ?, shape: ?, batch\_size: ?, optimizer: ?\}}\\[0.25em]
\textcolor{blue}{\textbf{to achieve}}\\
\texttt{Y = \{power: minimize, runtime: minimize\}}
}
& \cell{%
\texttt{X = depth = 7, batch\_size = 256, shape = rectangle\_residual, optimizer = Adam.}\\
Confidence: High (NLL: 0.00, OOD: 0.00, OOS: 0.00, MD: 0.00)
}\\ \hline

& CoMD
& \cell{%
\textcolor{blue}{\textbf{Recommend}} a configuration\\
\texttt{X = \{Bw\_level: ?, power\_cap: ?, app: CoMD\}}\\[0.25em]
\textcolor{blue}{\textbf{to achieve}}\\
\texttt{Y = \{perf\_variation: minimize, runtime: minimize\}}
}
& \cell{%
\ankur{fix this}
\texttt{X = \{algorithm = rand, num\_nodes\_req = 8\}}\\
Confidence: High (NLL: 0.10, OOD: 0.05, OOS: 0.06, MD: 0.04)
}\\ \cline{2-4}

& FT
& \cell{\textcolor{blue}{\textbf{Recommend}} a configuration\\
\texttt{X = \{bw\_level: ?, power\_cap: ?, app: CoMD\}}\\[0.25em]
\textcolor{blue}{\textbf{to achieve}}\\
\texttt{Y = \{power: minimize, runtime: minimize\}}}
& \cell{\texttt{bw\_level = 3, power\_cap = 112, runtime = 26.74, thread\_count = 20.}
Confidence: High (NLL: 0.00, OOD:
0.01, OOS: 0.00, MD: 0.00)}\\ \cline{2-4}

& HotPerfCloud
& \cell{
Recommend a configuration where
X = {ReqCPUS: ?, AllocCPUS: ?,
NCPUS: ?, NNode: ?, AllocNode: ?, is\_gpu: True}
to achieve
Y = {job\_state: COMPLETED, RlapsedRaw: minimized, CPUTimeRaw: minimized}
}
& \cell{\ankur{check the formation} NCPUS = 19.2, NNode = 1.0, AllocCPUS 
= 6.0, AllocNode = 1.0, ReqCPUS = 6.0. \\
Confidence: High(NLL: 0.07, OOD: 0.00, OOS: 0.04, MD: 0.03)}\\ \cline{2-4}

& F-Data
& \cell{---}
& \cell{---}\\ \cline{2-4}

& MIT Supercloud
& \cell{---}
& \cell{---}\\ \cline{2-4}

& MPI I/O Dataset
& \cell{Recommend me a configuration where X = {elements; ?, topology: ?, trial: ?, algo = "mvapich2"} to achieve Y = {cg\_residual: minimized}}
& \cell{
\ankur{rerun it by other algorithm}
elements = 9216.0, trial = 86, topology = torus-2-2-4. 0.00, 0.08, 0.16, 0.06 High}\\ \cline{2-4}

& Fresco
& \cell{X = {nhosts: ?, ncores: ?, queue: ?, host: ?}
to achieve
Y = {exitcode: ``COMPLETED", value\_cpuuser: ``minimize", ``timelimit": minimize}}
& \cell{\ankur{rerun it removing}}\\ \cline{2-4}
\hline

% ------------------ MODIFY ------------------
\multirow{6}{*}{\texttt{\textbackslash modify}}
& Monet
& \cell{%
\textcolor{blue}{\textbf{Modify}}\\
\texttt{X = \{X+\_*\_CREDIT\_STALL: x $\rightarrow$ 2x, X+\_*\_INQ\_STALL: x $\rightarrow$ 2x\}}\\[0.25em]
\textcolor{blue}{\textbf{to achieve}}\\
\texttt{Y = \{Z+\_*\_CREDIT\_STALL: reduce by 20\%\}}
}
& \cell{\texttt{Z-\_SAMPLE\_GEMINI\_LINK\_INQ\_STALL $\downarrow$ 93.8\%, nettopo\_mesh\_coord\_Y $\downarrow$ 7.14\%} \\
 Confidence: High (NLL: 0.00, OOD:
0.04, OOS: 0.00, MD: 0.00)}\\ \cline{2-4}

& PM100
& \cell{%
\textcolor{blue}{\textbf{Modify}}\\
\texttt{X = cores\_per\_task: ?, num\_cores\_req: ?, num\_nodes\_req: ?,
 mem\_req, time\_limit: ?, num\_gpus\_req: 16, job\_state: Completed }\\[0.25em]
\textcolor{blue}{\textbf{to achieve}}\\
\texttt{Y = \{node\_power\_consumption: reduce by 10\%\, \{mem\_power\_consumption: reduce by 10\%\, \{cpu\_power\_consumption: reduce by 10\%\}}
}
& \cell{cores\_per\_task: 68\% $\downarrow$, memory\_alloc: 65\%$\downarrow$ \\ Confidence: Moderate (NLL: 0.07, OOD:
0.04, OOS: 0.40, MD: 0.02)
}\\ \cline{2-4}

& Butter-E
\ankur{need to check again}
& \cell{%
\textcolor{blue}{\textbf{Modify}} we change \texttt{X = \{depth: old $\rightarrow$ 2 * old, is\_gpu = True, dataset = 'adult', shape: ?, batch\_size: ?, optimizer: ?\}}.\\
How would that affect \texttt{Y = \{power, run\_time\}}?
}
& \cell{

\texttt{shape: 
rectangle → rectangle\_residual.\\
Confidence: High(NLL: 0.01, OOD:
0.00, OOS: 0.03, MD: 0.01)}

}\\ \cline{2-4}

& CoMD
& \cell{%
\textcolor{blue}{\textbf{Modify}}\\
\texttt{X = \{Bw\_level: ?, power\_cap: ?, app: CoMD\}}\\[0.25em]
\textcolor{blue}{\textbf{to achieve}}\\
\texttt{Y = \{perf\_variation: reduce by 10\%\}}
}
& \cell{%
\texttt{node\_count: 4096 → 2026, power\_cap: 64 → 92 \\ High Confidence (NLL: 0.00, OOD: 0.02, OOS: 0.20, MD: 0.04)}
}\\ \cline{2-4}

& FT
& \cell{%
\textcolor{blue}{\textbf{Modify}}\\
\texttt{X = \{algorithm: ?, app: FT\}}\\[0.25em]
\textcolor{blue}{\textbf{to achieve}}\\
\texttt{Y = \{perf\_variation: reduce by 10\%\}}
}
& \cell{%
\texttt{algorithm: rand $\rightarrow$ spr}\\
Confidence: High (NLL: 0.02, OOD: 0.00, OOS: 0.07, MD: 0.06)
}\\ \cline{2-4}

& HotPerfCloud
& \cell{%
\textcolor{blue}{\textbf{Modify}}\\
\texttt{X = \{ReqCPUS: 4 $\rightarrow$ ?, AllocCPUS: 4 $\rightarrow$ ?, NCPUS: 4 $\rightarrow$ ?, NNode: 1 $\rightarrow$ ?, AllocNode: 1 $\rightarrow$ ?, is\_gpu: True\}}\\[0.25em]
\textcolor{blue}{\textbf{to achieve}}\\
\texttt{Y = \{job\_state: FAILED $\rightarrow$ COMPLETED\}}
}
& \cell{---}\\
\hline

% ------------------ WHATIF ------------------
\multirow{6}{*}{\texttt{\textbackslash whatif}}
& Monet
& \cell{%
\textcolor{blue}{\textbf{What if we change}}\\
\texttt{X = \{X+\_SAMPLE\_GEMINI\_LINK\_CREDIT\_STALL: old $\rightarrow$ new, X+\_SAMPLE\_GEMINI\_LINK\_INQ\_STALL: old $\rightarrow$ new, nettopo\_mesh\_coord\_X: ?, nettopo\_mesh\_coord\_Y: ?, nettopo\_mesh\_coord\_Z: ?\}}\\[0.25em]
\textcolor{blue}{\textbf{how would that affect}}\\
\texttt{Y = \{X+\_SAMPLE\_GEMINI\_LINK\_INQ\_STALL: minimize, X+\_SAMPLE\_GEMINI\_LINK\_CREDIT\_STALL: minimize, X+\_SAMPLE\_GEMINI\_LINK\_USED\_BW: minimize\}}?
}
& \cell{\texttt{nettopo\_mesh\_coord\_Z: 4.0 $\rightarrow$ 19.0, 
nettopo\_mesh\_coord\_Y: 3.0 $\rightarrow$ 16.0} \\ Confidence: High {NLL: 0.00, OOD: 0.00, OOS: 0.03, Composite Score: 0.00}}\\ \cline{2-4}

& PM100
& \cell{%
\textcolor{blue}{\textbf{What if we change}}\\
\texttt{X = \{num\_gpu\_req: old $\rightarrow$ 2 * old, job\_state = COMPLETED\}}\\[0.25em]
\textcolor{blue}{\textbf{how would that affect}}\\
\texttt{Y = \{node\_power\_consumption, mem\_power\_consumption, cpu\_power\_consumption}}?
& \cell{num\_cores\_req: 5\% $\uparrow$, \\num\_cores\_alloc: 5\% $\uparrow$ \\ Confidence: High {NLL: 0.00, OOD: 0.00, OOS: 0.00, Composite Score: 0.00}}\\ \cline{2-4}

& Butter-E
\ankur{need to check again. post after modify is checked}
& \cell{%
\textcolor{blue}{\textbf{What if we change}}\\
\texttt{X = \{depth: old $\rightarrow$ 2 * old, is\_gpu = True, dataset = adult\}}\\[0.25em]
\textcolor{blue}{\textbf{how would that affect}}\\
\texttt{Y = \{power, run\_time\}}?
}
& \cell{---}\\ \cline{2-4}

& CoMD
& \cell{%
\textcolor{blue}{\textbf{What-if we change}}\\
\texttt{X = \{app: CoMD, algorithm: ``rand'' $\rightarrow$ ``pak''\}}\\[0.25em]
\textcolor{blue}{\textbf{how will it affect}}\\
\texttt{Y = \{perf\_variation\}?
}}
& \cell{%
\texttt{
\texttt{perf\_variation: 92.13\% $\downarrow$}
}\\
}\\ \cline{2-4}

& FT
& \cell{%
\textcolor{blue}{\textbf{What-if we change}}\\
\texttt{X = \{app: FT, algorithm: ``rand'' $\rightarrow$ ``pak''\}}\\[0.25em]
\textcolor{blue}{\textbf{how will it affect}}\\
\texttt{Y = \{perf\_variation, run\_time\}}?
}
& \cell{%
\texttt{Y increases: perf\_variation $\uparrow$ 8.4\%, run\_time $\uparrow$ 12.1\%}\\
}\\ \cline{2-4}

& HotPerfCloud
& \cell{%
\textcolor{blue}{\textbf{What-if we change}}\\
\texttt{X = \{ReqCPUS: old $\rightarrow$ new, AllocNode: old $\rightarrow$ new, is\_gpu: True\}}\\[0.25em]
\textcolor{blue}{\textbf{how would that affect}}\\
\texttt{Y = \{job\_state: FAILED $\rightarrow$ COMPLETED\}}?
}
& \cell{---}\\
\hline
\end{longtable}
