# Supplementary material for: COMPASS: A Unified Decision-Intelligence System for Navigating Performance Trade-off in HPC
Source: arXiv:2604.22688 source file (2026-04-27)
Supplement: Supplementary file 2 [file appendix2.tex]

\begin{tiny}
\begin{longtable}{|p{0.08\textwidth}|p{0.55\textwidth}|p{0.33\textwidth}|}
\caption{All queries and answers.}
\label{tab:results-summary} \\

\hline
\parbox{1cm}{\centering \textbf{Dataset}} & 
\parbox{6cm}{\centering \textbf{Query}} & 
\parbox{3cm}{\centering \textbf{Response}} \\ \hline
\endfirsthead

\multicolumn{3}{c}%
{{\bfseries Table \thetable\ (continued)}} \\
\hline
\parbox{1cm}{\centering \textbf{Dataset}} & 
\parbox{6cm}{\centering \textbf{Query}} & 
\parbox{3cm}{\centering \textbf{Response}} \\ \hline
\endhead

\hline \multicolumn{3}{r}{{Continued on next page}} \\ \hline
\endfoot

\hline
\endlastfoot

% ---------------------- RECO ------------------------
\multicolumn{3}{|c|}{{\tablecellbl{\textbf{\reco}}}}\\\hline

Monet  &
\cell{
\textcolor{blue}{\textbf{Recommend a configuration where}}
\texttt{X = \{nettopo\_mesh\_coord\_Z: ?, nettopo\_mesh\_coord\_Y: ?, nettopo\_mesh\_coord\_X: ?\}}
\textcolor{blue}{\textbf{to achieve}}
\texttt{Y = \{X+\_SAMPLE\_GEMINI\_LINK\_INQ\_STALL: minimize, X+\_SAMPLE\_GEMINI\_LINK\_CREDIT\_STALL: minimized, X+\_SAMPLE\_GEMINI\_LINK\_USED\_BW: minimized\}}
} &
\cell{
\texttt{X = \{nettopo\_mesh\_coord\_Z = 19.0, nettopo\_mesh\_coord\_Y = 11.0, nettopo\_mesh\_coord\_X = 22.0\}}
}\\ \hline

PM100  &
\cell{
\textcolor{blue}{\textbf{Recommend a configuration where}}
\texttt{X = \{cores\_per\_task: ?, num\_cores\_req: ?, num\_nodes\_req: ?, mem\_req: ?, time\_limit: ?\}}
\textcolor{blue}{\textbf{to achieve}}
\texttt{Y = \{node\_power\_consumption: minimized, mem\_power\_consumption: minimized, cpu\_power\_consumption: minimized, job\_state: completed, num\_gpus\_req = 4\}}
} &
\cell{
\texttt{\{cores\_per\_task: 1, num\_cores\_req: 4, num\_nodes\_req: 1, mem\_req: 7, time\_limit: 30\}}
}\\ \hline

Butter-E  &
\cell{
\textcolor{blue}{\textbf{Recommend a configuration where}}
\texttt{X = \{is\_gpu: True, dataset: ``mnist", depth: ?, shape: ?, batch\_size: ?, optimizer: ?\}}
\textcolor{blue}{\textbf{to achieve}}
\texttt{Y = \{power: minimized, runtime: minimized\}}
} &
\cell{
\texttt{\{is\_gpu: True, dataset: ``mnist", depth: 7, shape: rectangle\_residual, batch\_size: 256, optimizer: Adam\}}
}\\ \hline

CoMD  &
\cell{
\textcolor{blue}{\textbf{Recommend a configuration where}}
\texttt{X = \{bw\_level: ?, power\_cap: ?, app: CoMD\}}
\textcolor{blue}{\textbf{to achieve}}
\texttt{Y = \{perf\_variation: minimize, runtime: minimize\}}
} &
\cell{
\texttt{X = \{bw\_level: 1, power\_cap: 64, app: CoMD\}}
}\\ \hline

FT  &
\cell{
\textcolor{blue}{\textbf{Recommend a configuration where}}
\texttt{X = \{bw\_level: ?, power\_cap: ?, app: FT\}}
\textcolor{blue}{\textbf{to achieve}}
\texttt{Y = \{perf\_variation: minimize, runtime: minimize\}}
} &
\cell{
\texttt{bw\_level = 3, power\_cap = 112, app: FT}
}\\ \hline

\cell{
HotPerf\newline-Cloud
} &
\cell{
\textcolor{blue}{\textbf{Recommend a configuration where}}
\texttt{X = \{ReqCPUS: ?, NCPUS: ?, NNode: ?, is\_gpu: True\}}
\textcolor{blue}{\textbf{to achieve}}
\texttt{Y = \{job\_state: COMPLETED, ElapsedRaw: minimized\}}
} &
\cell{
\texttt{ReqCPUS: 3.0, NCPUS: 3.0, NNode: 1.0, is\_gpu: True}
}\\ \hline

F-Data & \cell{---} & \cell{---}\\ \hline
MIT \newline Supercloud & \cell{---} & \cell{---}\\ \hline

MPI I/O &
\cell{
\textcolor{blue}{\textbf{Recommend a configuration where}}
\texttt{X = \{elements: ?, topology: ?, trial: ?, algo: ?\}}
\textcolor{blue}{\textbf{to achieve}}
\texttt{Y = \{cg\_residual: minimized\}}
} &
\cell{
\texttt{elements = 9216.0, topology = "torus-2-2-4",  trial = 86, algo = "rab"}
}\\ \hline

Fresco &
\cell{
\textcolor{blue}{\textbf{Recommend a configuration where}}
\texttt{X = \{nhosts: ?, ncores: ?, queue: ?, host: ?\}}
\textcolor{blue}{\textbf{to achieve}}
\texttt{Y = \{exitcode: "COMPLETED", value\_cpuuser: minimize, timelimit: minimize\}}
} &
\cell{---}\\ \hline

% ---------------------- MODIFY ------------------------
\multicolumn{3}{|c|}{{\tablecellgr{\textbf{\modify}}}}\\\hline

Monet &
\cell{
\textcolor{blue}{\textbf{Modify}}
\texttt{X = \{X+\_*\_CREDIT\_STALL: x→2x, X+\_*\_INQ\_STALL: x→2x\}}
\textcolor{blue}{\textbf{to achieve}}
\texttt{Y = \{Z+\_*\_CREDIT\_STALL: reduce by 20\%\}}
} &
\cell{
\texttt{Z-\_SAMPLE\_GEMINI\_LINK\_INQ\_STALL ↓93.8\%, nettopo\_mesh\_coord\_Y ↓7.14\%}

}\\ \hline

PM100 &
\cell{
\textcolor{blue}{\textbf{Modify}}
\texttt{X = \{cores\_per\_task: ?, num\_cores\_req: ?, num\_nodes\_req: ?, mem\_req: ?, time\_limit: ?, num\_gpus\_req: 16, job\_state: Completed\}}
\textcolor{blue}{\textbf{to achieve}}
\texttt{Y = \{node\_power\_consumption, mem\_power\_consumption, cpu\_power\_consumption: reduced by 10\%\}}
} &
\cell{
\texttt{cores\_per\_task ↓68\%, memory\_alloc ↓65\%}
}\\ \hline

Butter-E &
\cell{
\textcolor{blue}{\textbf{Modify}}
\texttt{X = \{depth: ?, is\_gpu=True, dataset='adult', shape: ?, batch\_size: ?, optimizer: ?\}}
\textcolor{blue}{\textbf{to achieve}}
\texttt{Y = \{power: 10\% reduction, runtime: 10\% reduction\}}
} &
\cell{
\texttt{\{depth: 15, is\_gpu=True, dataset='adult', shape: "trapezoid', batch\_size: 256, optimizer: "Adam"\}}
}\\ \hline

CoMD &
\cell{
\textcolor{blue}{\textbf{Modify}}
\texttt{X = \{Bw\_level: ?, power\_cap: ?, app: CoMD\}}
\textcolor{blue}{\textbf{to achieve}}
\texttt{Y = \{perf\_variation: reduce by 10\%\}}
} &
\cell{
\texttt{node\_count: 4096→2026, power\_cap: 64→92}
}\\ \hline

FT &
\cell{
\textcolor{blue}{\textbf{Modify}}
\texttt{X = \{algorithm: ?, app: FT\}}
\textcolor{blue}{\textbf{to achieve}}
\texttt{Y = \{perf\_variation: reduce by 10\%\}}
} &
\cell{
\texttt{algorithm: rand→spr}\\
}\\ \hline

HotPerf\newline Cloud &
\cell{
\textcolor{blue}{\textbf{Modify}}
\texttt{X = \{ReqCPUS: 1→?, NCPUS: 3→?, NNode: 1→?, is\_gpu: True\}}
\textcolor{blue}{\textbf{to achieve}}
\texttt{Y = \{job\_state: FAILED→COMPLETED\}}
} &
\cell{\texttt{\{ReqCPUS: 1→1, NCPUS: 3→7, NNode: 1→1, is\_gpu: True\}}}\\ \hline

F-Data & \cell{---} & \cell{---}\\ \hline
MIT \newline Supercloud & \cell{---} & \cell{---}\\ \hline

MPI I/O &
\cell{
\textcolor{blue}{\textbf{Modify}}
\texttt{X = \{elements: ?, trial: ?, NP: ?, topology": "fattree-72\}}
\textcolor{blue}{\textbf{to achieve}}
\texttt{Y = \{cg\_residual: reduced by 10\%\}}
} &
\cell{
\texttt{elements = 9216.0, trial = 67, NP =  22,  topology = "torus-2-2-4"}
}\\ \hline

Fresco &
\cell{

} &
\cell{---}\\ \hline

% ---------------------- WHATIF ------------------------
\multicolumn{3}{|c|}{{\tablecellor{\textbf{\whatif}}}}\\\hline

Monet &
\cell{
\textcolor{blue}{\textbf{What if we change}}
\texttt{X = \{X+\_SAMPLE\_GEMINI\_LINK\_CREDIT\_STALL, X+\_SAMPLE\_GEMINI\_LINK\_INQ\_STALL, nettopo\_mesh\_coord\_X, Y, Z\}}
\textcolor{blue}{\textbf{how would that affect}}
\texttt{Y = \{link stalls: minimize\}}?
} &
\cell{
\texttt{nettopo\_mesh\_coord\_Z: 4→19, nettopo\_mesh\_coord\_Y: 3→16}\\
}\\ \hline

PM100 &
\cell{
\textcolor{blue}{\textbf{What if we change}}
\texttt{X = \{num\_gpu\_req: old→2×old, job\_state=COMPLETED\}}
\textcolor{blue}{\textbf{how would that affect}}
\texttt{Y = \{node, mem, cpu power consumption\}}?
} &
\cell{
\texttt{num\_cores\_req ↑5\%, num\_cores\_alloc ↑5\%}\\
}\\ \hline

Butter-E & \cell{
\textcolor{blue}{\textbf{What if we change}}
\texttt{X = \{depth: old→2×old, is\_gpu: True, dataset: "adult"\}}
\textcolor{blue}{\textbf{how would that affect}}
\texttt{Y = \{power, runtime\}}?
}
& \cell{power: 0\% $\uparrow$, rutime: 3.41\% $\uparrow$}\\ \hline

CoMD &
\cell{
\textcolor{blue}{\textbf{What-if we change}}
\texttt{X = \{app: CoMD, algorithm: rand→pak\}}
\textcolor{blue}{\textbf{how will it affect}}
\texttt{Y = \{perf\_variation\}}?
} &
\cell{
\texttt{perf\_variation ↓92.13\%}
}\\ \hline

FT &
\cell{
\textcolor{blue}{\textbf{What-if we change}}
\texttt{X = \{app: FT, algorithm: rand→pak\}}
\textcolor{blue}{\textbf{how will it affect}}
\texttt{Y = \{perf\_variation, run\_time\}}?
} &
\cell{
\texttt{perf\_variation ↑8.4\%, run\_time ↑12.1\%}
}\\ \hline

HotPerf\newline Cloud &
\textcolor{blue}{\textbf{What-if we change}}
\texttt{X = \{ReqCPUS: old $\rightarrow$ 2* old, is\_gpu: True\}}
\textcolor{blue}{\textbf{how would that affect}}
\texttt{Y = \{job\_state: FAILED $\rightarrow$ COMPLETED\}}?
& 
\cell{
\texttt{req\_mem: 835.38\% $\uparrow$}
}\\ \hline

F-Data & \cell{---} & \cell{---}\\ \hline
MIT \newline Supercloud & \cell{---} & \cell{---}\\ \hline

MPI I/O &
\cell{
\textcolor{blue}{\textbf{What-if we chnage}}
\texttt{X = \{trial: x $\rightarrow$ 3*x, topology": "fattree-72" $\rightarrow$ fattree-16\}}
\textcolor{blue}{\textbf{how would that affect}}
\texttt{Y = \{cg\_residual\}}?
} &
\cell{
\texttt{"algo: smp\_rsag\_lr $\rightarrow$
ompi\_ring\_segmented"}
}\\ \hline

Fresco &
\cell{

} &
\cell{---}\\ \hline

\end{longtable}
\end{tiny}
